# Supplementary material for: Learning-based Inverse Rendering of Complex Indoor Scenes with Differentiable Monte Carlo Raytracing
Source: arXiv:2211.03017 ancillary file (2022-11-23)
Supplement: Supplementary file 1 [file supplementary.pdf]

# Supplementary Material: Learning-based Inverse Rendering of Complex Indoor Scenes with Differentiable Monte Carlo Raytracing


Jingsen Zhu
zhujingsen@zju.edu.cn
State Key Lab of CAD&CG, Zhejiang University
China

Fujun Luan
fluan@adobe.com
Adobe Research
USA

Yuchi Huo*
huo.yuchi.sc@gmail.com
State Key Lab of CAD&CG, Zhejiang University
Zhejiang Lab
China

Zihao Lin
zihaolin@zju.edu.cn
State Key Lab of CAD&CG, Zhejiang University
China

Zhihua Zhong
zhongzhihua@zju.edu.cn
State Key Lab of CAD&CG, Zhejiang University
China

Dianbing Xi
db.xi@zju.edu.cn
State Key Lab of CAD&CG, Zhejiang University
China

Jiaxiang Zheng
xuanfeng@qunhemail.com
KooLab, Manycore
China

Rui Tang
ati@qunhemail.com
KooLab, Manycore
China

Hujun Bao
bao@cad.zju.edu.cn
State Key Lab of CAD&CG, Zhejiang University
China

Rui Wang*
rwang@cad.zju.edu.cn
State Key Lab of CAD&CG, Zhejiang University
China



**ACM Reference Format:**
Jingsen Zhu, Fujun Luan, Yuchi Huo, Zihao Lin, Zhihua Zhong, Dianbing Xi, Jiaxiang Zheng, Rui Tang, Hujun Bao, and Rui Wang. 2022. Supplementary Material: Learning-based Inverse Rendering of Complex Indoor Scenes with Differentiable Monte Carlo Raytracing. In *SIGGRAPH Asia 2022 Conference Papers (SA '22 Conference Papers), December 6–9, 2022, Daegu, Republic of Korea.* ACM, New York, NY, USA, 6 pages. https://doi.org/10.1145/3550469.3555407


## 1 NETWORK ARCHITECTURE DETAILS

*Network structure of our material-geometry network.* , **MGNet**, is shown in Fig. 1. We share DenseNet121 [Huang et al. 2017] as the 2D CNN encoder backbone, which produces 5 levels of intermediate latent space features $X_1 \sim X_5$. 4 separate branches of decoders predicts albedo $A$, normal $N$, depth $D$, roughness $R$ and metallic $M_t$ with skip connections. Note that $R$ and $M_t$ is predicted by the same branch of decoder with 2-channel outputs respectively. We find that jointly predict roughness and metallic in one branch gives better results than separate into two branches. This may be because of the semantic correlations between these two material attributes.

*Network structure of our SSRT-based lighting network.* , is illustrated in Fig. 2. We use the first 4 layers of ResNet34 as the backbone of the CNN encoder, which produces a feature map $F$ of 1024 channels. After obtaining source point $\mathbf{s}$ in the scene by screen-space ray tracing, we project $\mathbf{s}$ onto the image coordinates $\pi(\mathbf{s})$ and extract a 1024-channel local feature from $F$. The MLP takes the local feature, as well as light direction $\mathbf{d}$ and diffuse albedo $K_d$, specular albedo $K_s$, and roughness $R$ on point $\pi(\mathbf{s})$. To increase data frequency, we incorporate fourier features [Tancik et al. 2020] to encode the G-Buffer values. The final MLP is an 8-layer 512-channel MLP with skip connection at the 4th layer.

*Network details of our out-of-view lighting network.* The global encoder is a ResNet34 CNN network followed by a global average pooling layer. The input image passed through the global encoder

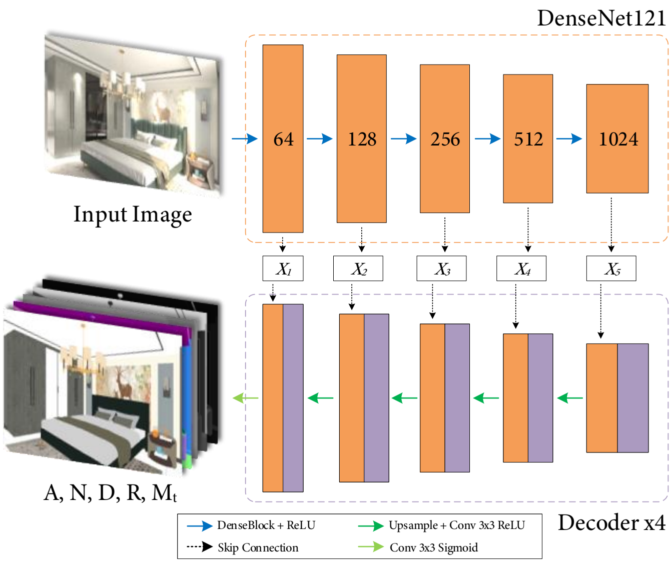


**Figure 1: Detailed architecture of MGNet.**

*Denotes corresponding author.


*SA '22 Conference Papers, December 6–9, 2022, Daegu, Republic of Korea*
2022. ACM ISBN 978-1-4503-9470-3/22/12…$15.00
https://doi.org/10.1145/3550469.3555407

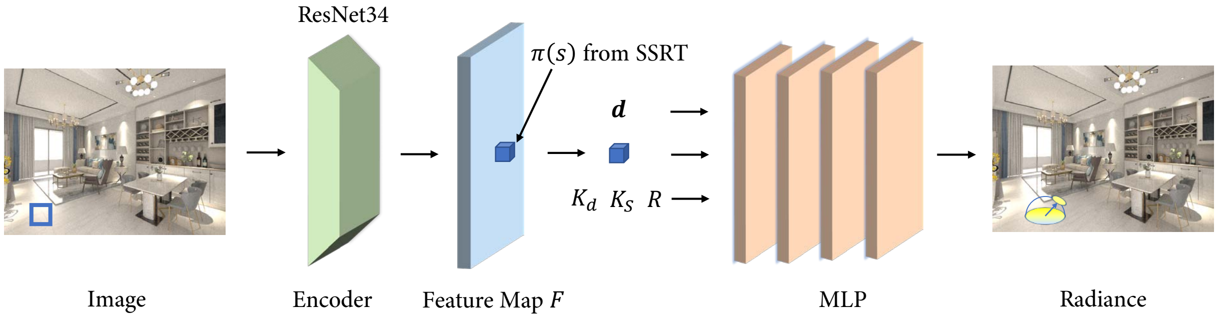


**Figure 2: Detailed architecture of our SSRT-based lighting prediction network.**

becomes a 512-channel global feature. The NeRF network we used is a 4-layer MLP with 64 as its latent channel size. The weights and biases of the 4-layer MLP are predicted by 8 separate branches of hypernetwork which takes the global feature as input. Each hypernetwork has the same structure of a 3-layer MLP with 1024 as its latent channel size.

*Implementation and training details.* We implement our network model with Pytorch [2019]. We train our network using 8 NVIDIA Tesla V100 GPUs, and use Adam [2014] optimizer with an initial learning rate of $1e$-4 for **MGNet** and $1e$-5 for **LightNet**. For **MGNet**, the training set contains 44950 images, and we reserve 4980 images for evaluation. For **LightNet** (SSRT-based network and out-of-view network), we use 1000 scenes for training, and each scene contains 400 spatially-varying HDR environment maps. We use 90% scenes for training, and the rest are reserved for evaluation. For the Monte Carlo rendering layer, we pre-compute 256 sampling directions on the surface point of each pixel using GGX importance sampling, and query the ground-truth radiance of each sample. The radiance-direction pairs are cached and used as training data to supervise our network. The spatial resolution of sampled pixels is $120 \times 160$.

## 2 DETAILS OF INDOOR DATASET

The InteriorVerse dataset contains 4176 indoor scenes, which are designed by professional indoor designers. Each scene contains 1 manually-placed camera as well as several automatic generated cameras. We use the heuristic camera generating method proposed by [Genova et al. 2017], which maximizes the number and pixel occupancy of object categories in the output views. Images in the dataset are rendered by a commercial GPU-accelerated path tracer with NVIDIA RTX 3090. InteriorVerse dataset provides per-pixel **albedo, normal, depth, roughness, metallic** and spatially-varying **environment maps** as lighting representations. The 3D locations related to each environment map are randomly sampled in *view space* coordinates and will also be provided.

## 3 DETAILS OF TRAINING LOSS

### 3.1 Material-Geometry Network

We use combination of a $L_2$ loss and a perceptual loss [Johnson et al. 2016] to avoid blurriness. For the perceptual loss $\mathcal{L}_\text{p}$, we use the output from a pretrained `relu_3_3` layer from a VGG-16 network. We find that despite non-photorealistic albedo/normal/material maps, the perceptual loss still works well and helps to preserve semantic consistency.

For the albedo, similar to [Li et al. 2020], we use a scale invariant loss due to the ambiguity between color and light intensity. We define

$$\mathcal{L}_\text{albedo} = \|A - c\hat{A}\|_2 + \lambda_\text{p}\mathcal{L}_\text{p}(A, c\hat{A}), \quad (1)$$

where $c = \arg\min_c \|A - c\hat{A}\|_2^2 = \frac{\sum_p \hat{A}_p \cdot A_p}{\hat{A}_p \cdot \hat{A}_p}$ is the scale factor computed by least square regression and $\lambda_\text{p}$ is the scale factor of perceptual loss.

For normals, we normalize the prediction and use a $L_1$ angular error as well as perceptual loss:

$$\mathcal{L}_\text{normal} = \left\| 1 - N \cdot (\frac{\hat{N}}{\|\hat{N}\|}) \right\|_1 + \lambda_\text{p}\mathcal{L}_\text{p}(N, \hat{N}). \quad (2)$$

For roughness and metallic, we use a $L_2$ as well as a perceptual loss. Note that roughness and metallic are single-channel predictions, so we expand it into a 3-channel gray image before inputting into the VGG network.

$$\mathcal{L}_\text{material} = \|M - \hat{M}\|_2 + \lambda_\text{p}\mathcal{L}_\text{p}(R, \hat{R}) + \lambda_\text{p}\mathcal{L}_\text{p}(M_t, \hat{M}_t). \quad (3)$$

For depth, we follow [Li et al. 2020] to use a scale-invariant log-encoded $L_2$ loss to tackle high-dynamic-range issues:

$$\mathcal{L}_\text{depth} = \| \log(D+1) - \log(c\hat{D}+1)\|_2^2, \quad (4)$$

where $c = \frac{\sum_p \hat{D}_p \cdot D_p}{\hat{D}_p \cdot \hat{D}_p}$ is the scale factor of least square regression.

To sum up, the final loss is the weighted sum of all the losses mentioned above:

$$\mathcal{L}_\text{MGNet} = \lambda_a\mathcal{L}_\text{albedo} + \lambda_n\mathcal{L}_\text{normal} + \lambda_m\mathcal{L}_\text{material} + \lambda_d\mathcal{L}_\text{depth}. \quad (5)$$

In practice, we set $\lambda_\text{p} = 0.02$ and other weights to 1 for all results.

### 3.2 Lighting Network

*Direct supervision.* With ground truth lighting we can directly supervise our model. However, since the light field is high dynamic range, the color distribution can span many orders of magnitude. Standard $L_2$ loss applied in HDR color space will be completely dominated by errors in bright areas and fail to learn high-frequency details in dark areas. We apply the same HDR supervision loss function as in [Mildenhall et al. 2021]:

$$\mathcal{L}_\text{light} = \left\| \frac{\hat{L}_i - L_i}{\text{sg}(\hat{L}_i) + \epsilon} \right\|_2, \quad (6)$$

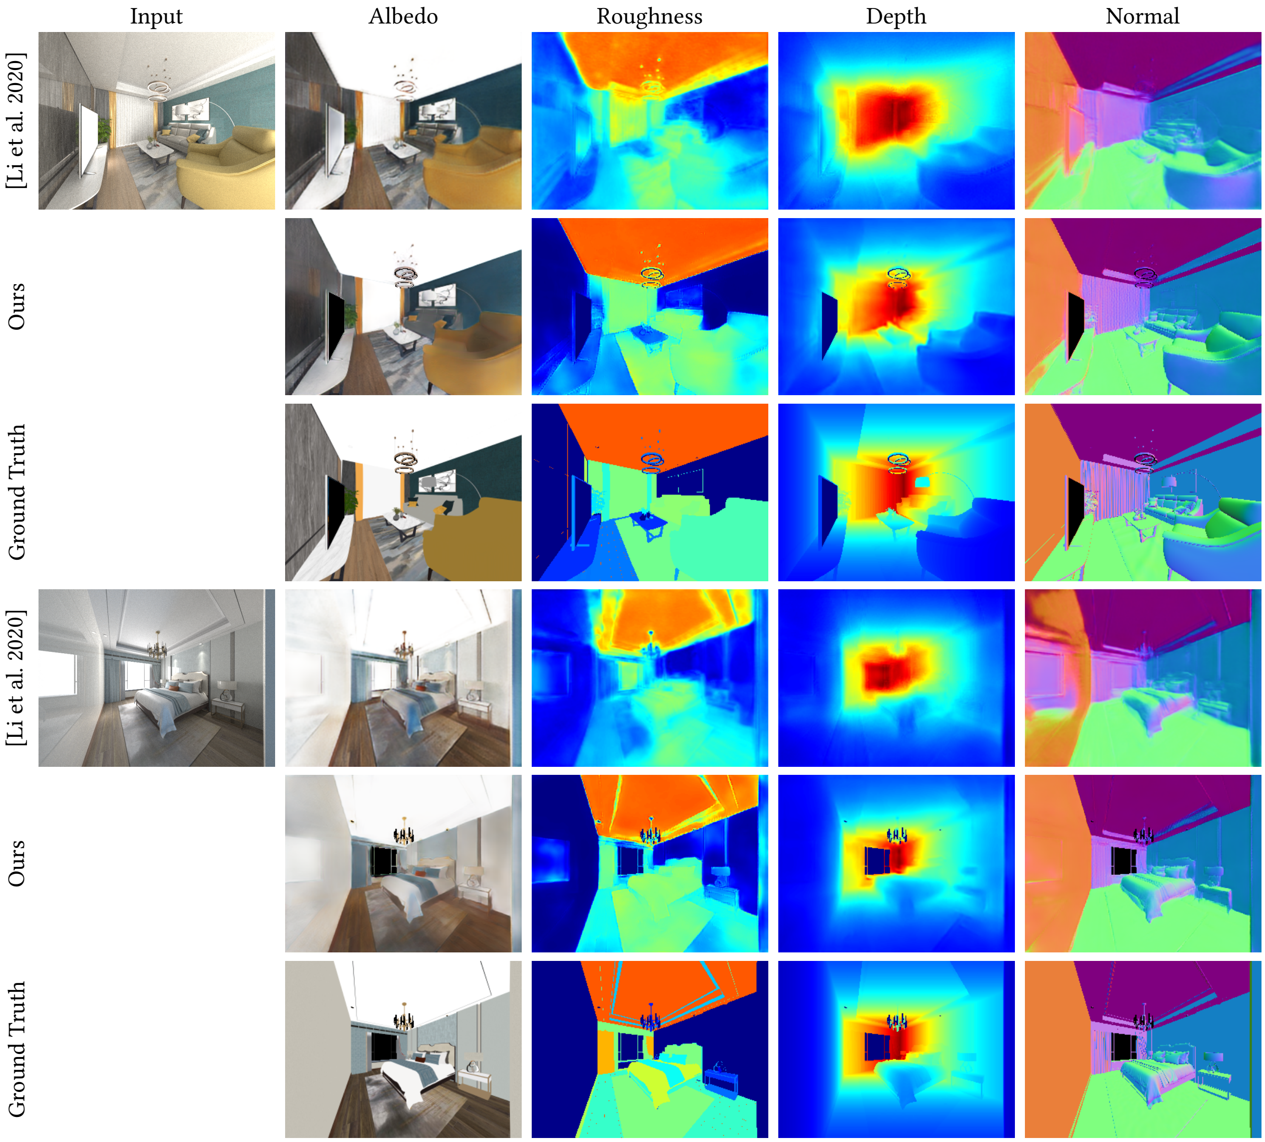


**Figure 3: More results of geometry and BRDF estimation on synthetic dataset.**

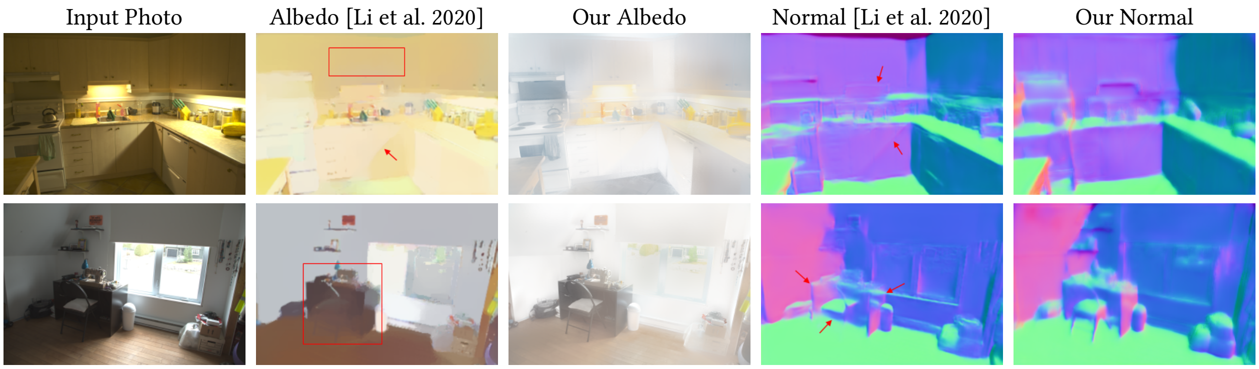


**Figure 4: More results of normal and albedo estimation on real images. [Li et al. 2020]'s artifacts are highlighted.**

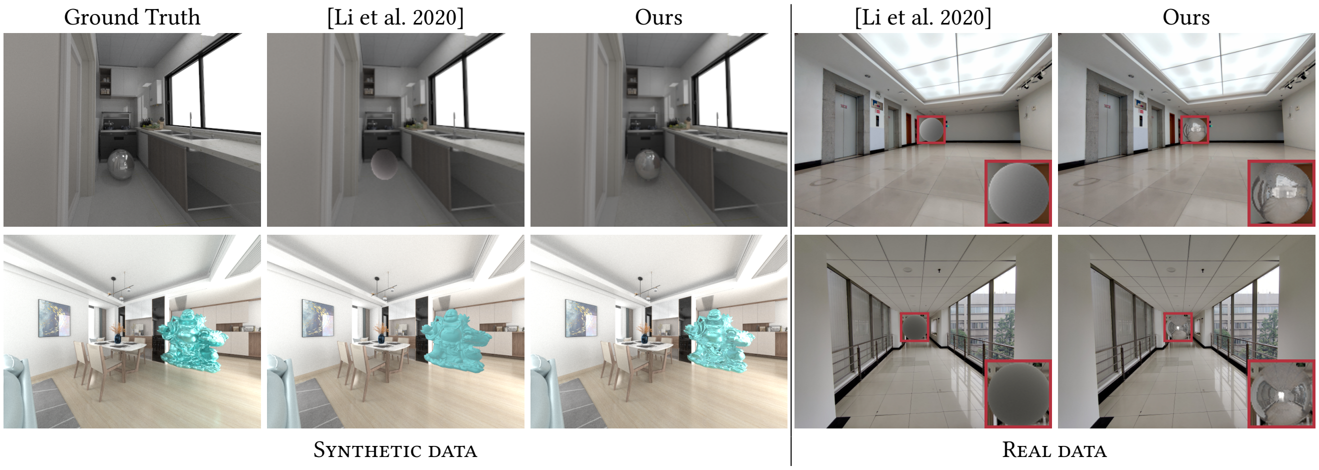


**Figure 5: Qualitative comparison of object insertion results on synthetic dataset and real-world images.**

where sg(·) indicates stop-gradient to prevent the denominator from influencing the loss gradient during backpropagation, and $\epsilon = 10^{-3}$ is the epsilon value to prevent division by zero.

*Re-rendering loss.* With our Monte Carlo importance sampling rendering layer, we can use the predicted material, geometry and lighting to re-render an image $\hat{I}$ and enforce its consistency with the original input image $I$. Specifically, for each pixel $\mathbf{p}$ of image $I$ (the corresponding view direction is $\mathbf{v}$), we can importance sample $N$ incident directions $\{\mathbf{d}_i\}$ along with the BRDF value $\{f_r(\mathbf{v}, \mathbf{d}_i)\}$ and PDF value $\{p(\mathbf{v}, \mathbf{d}_i)\}$ according to surface normal, albedo and roughness. Then, we query each radiance $L_i(\mathbf{p}, \mathbf{d}_i)$ from our network and use Monte Carlo integration (Eq. 7 in main paper) to produce $\hat{I}$. We use $L_2$ loss as the re-rendering loss $\mathcal{L}_{\text{re-render}} = \|\hat{I} - I\|_2$.

The final loss is the weighted sum of direct light supervision loss and re-rendering loss:

$$\mathcal{L}_{\textbf{LightNet}} = \mathcal{L}_{\text{light}} + \lambda_r \mathcal{L}_{\text{re-render}} \tag{7}$$

In practice, we set $\lambda_r = 3$.

## 4 ADDITIONAL EXPERIMENT RESULTS

*Qualitative results of material and geometry estimation on synthesis data.* Fig. 3 shows results between our method and [Li et al. 2020] (*finetuned on* InteriorVerse). Our method outperforms [Li et al. 2020], with sharper edges and better semantic consistency.

*Qualitative results of material and geometry estimation on real-world images.* We test our method on real-world images from Garon et al. [Garon et al. 2019] in Fig. 4. Although without ground truth, we can observe better intrinsic decomposition than prior works from visual comparison. For albedo estimation, in the first row of images, our method successfully extracts colors from yellow light conditions, while [Li et al. 2020] results in overly yellowish estimations. For normal estimation, in the second row of images, [Li et al. 2020] made wrong normal predictions at the desk and the chair, while our method makes more physically correct predictions.

*Evaluations on re-rendered image.* Fig. 7 shows qualitative results on re-render results using predicted lighting information on example scenes in our dataset. In order to emphasize the advantages of our Monte Carlo importance sampling render layer on specular reflections, we select scenes containing surfaces with high glossiness.

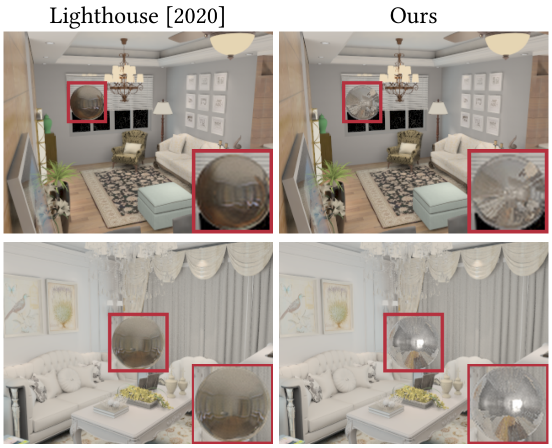


**Figure 6: Qualitative comparison of object insertion results on Lighthouse's test set. Lighthouse takes a stereo pair of images as input.**

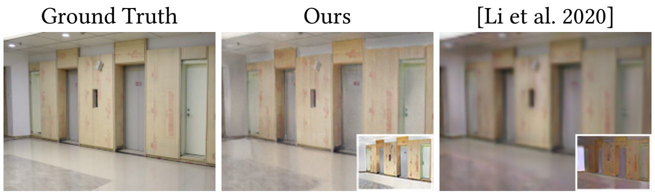


**Figure 7: Re-render results on real data with predicted albedo (insets).**

Our method significantly outperforms Li et al. [2020] in both lighting estimation and rendering, especially on glossy and specular

surfaces. In Fig. 7, we show the re-rendering results on real data. We choose a photo containing a *specular floor* that shows reflected wall on it to demonstrate the superior quality from our Monte Carlo rendering layer. Li et al. [2020] turns out a blurry image, while our method successfully reconstruct even the specular reflections on the floor. We also show the corresponding albedo prediction as insets, to demonstrate that our **MGNet** successfully extract material color from lighting effects, while Li et al. [2020]'s albedo baked in the reflections on the floor. As a result, our reconstructed reflections on the floor is contributed by both precise material and lighting predictions instead of incomplete intrinsic decomposition.

*Qualitative results of virtual object insertions.* Fig. 5 shows more results on virtual object insertions to synthetic and real-world images. [Li et al. 2020] still fails in this task, due to its low-frequency lighting estimation, leading to diffuse-like appearance. Our method preserves high-frequency angular reflections and is consistent with the surrounding environment.

Fig. 6 compares more results of our method and Lighthouse [2020]. We use the same experimental settings as in main text, using Lighthouse's test set without finetuning our network. We outperform Lighthouse, with more consistent reflection to the surroundings on the sphere and more variation in lighting intensity.

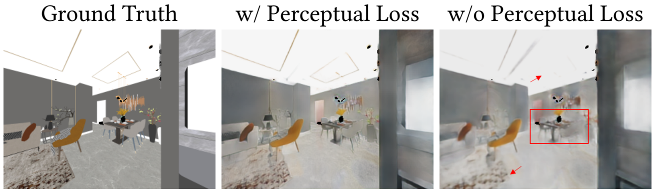


**Figure 8: Qualitative comparison of predicted albedo with our model trained with or without perceptual loss.**

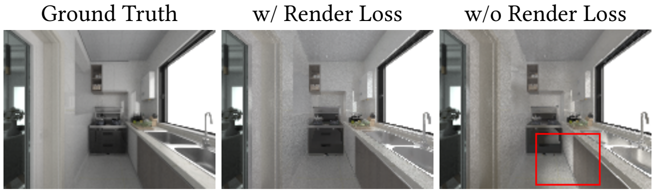


**Figure 9: Qualitative comparison of re-rendered image with our model trained with or without re-render loss.**

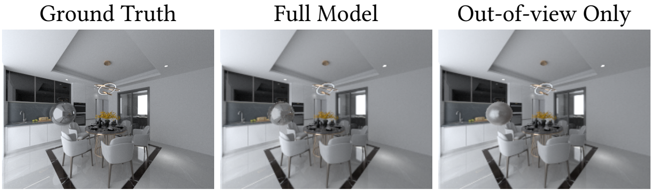


**Figure 10: Qualitative comparison of chrome ball insertion between using full model combined with uncertainty and only using out-of-view network. Zoom in for details.**

*Qualitative results of scene edit.* We further demonstrate another augmented reality application: scene edit. [Li et al. 2020] can perform material edit on diffuse surfaces, but their low-frequency lighting prediction quality and biased rendering layer limit their capabilities on specular surfaces. In contrast, our physically-based MC rendering layer enables correct re-render results on specular surfaces. As shown in Fig. 11, we edit albedo, roughness and metallic on the original images. The first row changes the non-metal glossy floor into a metallic floor (roughness unchanged), as well as changing the albedo color. The second row increases the metallic of the rough wall, showing rough-metal reflection effects. Our method both produces photorealistic results.

## 4.1 Ablation Studies

*Effects of perceptual loss.* We ablate our training choices of the material-geometry network in Fig. 8. From the results, it turns out that the model trained without perceptual loss predicts blurry results, and high-frequency details such as carpet textures and ceiling frames are lost. In contrast, the model trained with perceptual loss preserves clear semantic boundaries and is capable of predicting some of the high-frequency details. This shows the benefits of our perceptual loss design, which helps the network to learn semantic information of the scene.

*Effects of re-render loss.* We ablate our training choices of the lighting network in Fig. 9, comparing the effects of our re-render loss design. It turns out that lacking re-render loss leads to artifacts of shadows in the re-rendered image, confirming the effectiveness of re-render loss.

*Comparison between out-of-view network and full model.* We ablate between using only out-of-view network predictions and using full model predictions combined with uncertainty. We insert a chrome ball into an image to demonstrate the difference in reflections in Fig. 10. The reflections in out-of-view-only prediction are blurry and only contain angular intensity variance, while those in full-model prediction contain more high-frequency details. This proves that the SSRT component in **LightNet** enhances the light prediction quality.

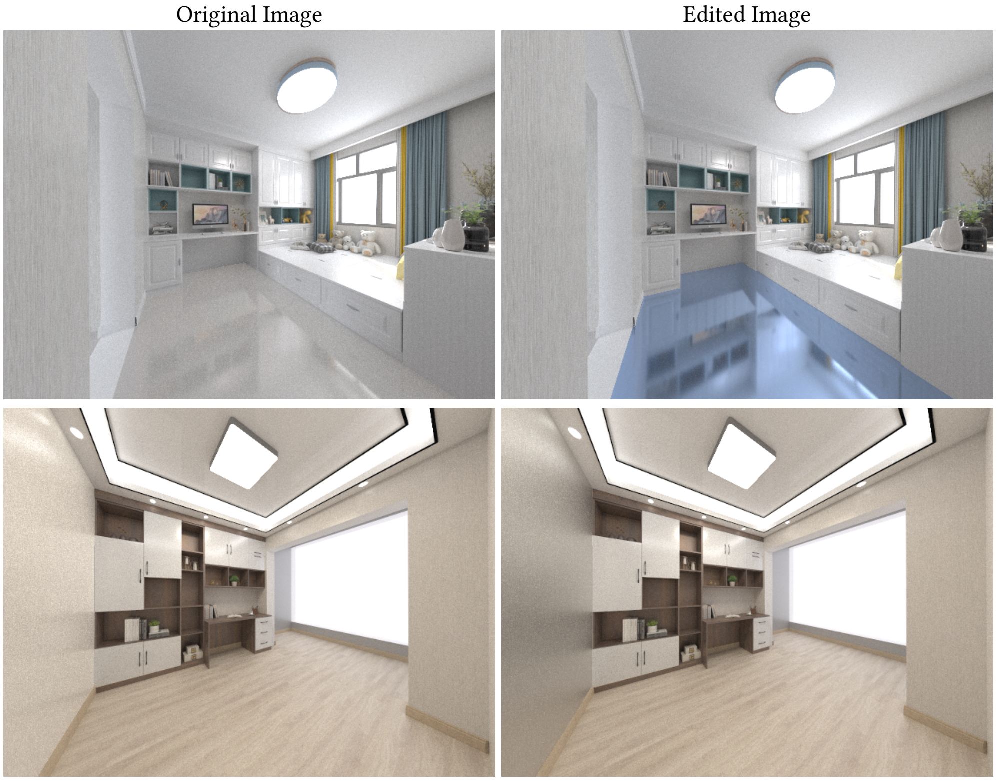


**Figure 11: Qualitative results of scene material edit, changing albedo, roughness and metallic on the surfaces.**

## REFERENCES

Mathieu Garon, Kalyan Sunkavalli, Sunil Hadap, Nathan Carr, and Jean-François Lalonde. 2019. Fast spatially-varying indoor lighting estimation. In *Proceedings of the IEEE/CVF Conference on Computer Vision and Pattern Recognition*. 6908–6917.

Kyle Genova, Manolis Savva, Angel X Chang, and Thomas Funkhouser. 2017. Learning where to look: Data-driven viewpoint set selection for 3d scenes. *arXiv preprint arXiv:1704.02393* (2017).

Gao Huang, Zhuang Liu, Laurens Van Der Maaten, and Kilian Q Weinberger. 2017. Densely connected convolutional networks. In *Proceedings of the IEEE conference on computer vision and pattern recognition*. 4700–4708.

Justin Johnson, Alexandre Alahi, and Li Fei-Fei. 2016. Perceptual losses for real-time style transfer and super-resolution. In *European conference on computer vision*. Springer, 694–711.

Diederik P Kingma and Jimmy Ba. 2014. Adam: A method for stochastic optimization. *arXiv preprint arXiv:1412.6980* (2014).

Zhengqin Li, Mohammad Shafiei, Ravi Ramamoorthi, Kalyan Sunkavalli, and Manmohan Chandraker. 2020. Inverse rendering for complex indoor scenes: Shape, spatially-varying lighting and svbrdf from a single image. In *Proceedings of the IEEE/CVF Conference on Computer Vision and Pattern Recognition*. 2475–2484.

Ben Mildenhall, Peter Hedman, Ricardo Martin-Brualla, Pratul Srinivasan, and Jonathan T Barron. 2021. NeRF in the Dark: High Dynamic Range View Synthesis from Noisy Raw Images. *arXiv preprint arXiv:2111.13679* (2021).

Adam Paszke, Sam Gross, Francisco Massa, Adam Lerer, James Bradbury, Gregory Chanan, Trevor Killeen, Zeming Lin, Natalia Gimelshein, Luca Antiga, et al. 2019. Pytorch: An imperative style, high-performance deep learning library. *Advances in neural information processing systems* 32 (2019).

Pratul P Srinivasan, Ben Mildenhall, Matthew Tancik, Jonathan T Barron, Richard Tucker, and Noah Snavely. 2020. Lighthouse: Predicting lighting volumes for spatially-coherent illumination. In *Proceedings of the IEEE/CVF Conference on Computer Vision and Pattern Recognition*. 8080–8089.

Matthew Tancik, Pratul Srinivasan, Ben Mildenhall, Sara Fridovich-Keil, Nithin Raghavan, Utkarsh Singhal, Ravi Ramamoorthi, Jonathan Barron, and Ren Ng. 2020. Fourier features let networks learn high frequency functions in low dimensional domains. *Advances in Neural Information Processing Systems* 33 (2020), 7537–7547.
